# Supplementary material for: CyberEvolver: Structured Self-Evolution for Cybersecurity Agents On the Fly
Source: arXiv:2605.26195 source file (2026-06-16)
Supplement: Supplementary file 4 [file refiner_prompt_registry.tex]

% Generated by scripts/render_refiner_prompt_registry.py; do not edit by hand.
% Each group is rendered with \renderrefinerpromptcards{<group>}.
\makeatletter
\newcommand{\refinerpromptcard}[4]{%
  \terminalpromptfile{#1}{#2}{firstline=#3,lastline=#4}%
}
\newcommand{\renderrefinerpromptcards}[1]{%
  \@ifundefined{refinerpromptcards@#1}{%
    \PackageWarning{CyberEvolver}{No refiner prompt card group `#1'}%
  }{%
    \@nameuse{refinerpromptcards@#1}%
  }%
}

\@namedef{refinerpromptcards@compression}{%
  \refinerpromptcard{system_prompt_thought_obs_summarizer_chunk}{appendix/generated/prompt_skill.tex}{133}{175}%
  \refinerpromptcard{user_prompt_thought_obs_summarizer_chunk}{appendix/generated/prompt_skill.tex}{178}{235}%
}

\@namedef{refinerpromptcards@diagnosis}{%
  \refinerpromptcard{system_prompt_eureka}{appendix/generated/prompt_skill.tex}{242}{267}%
  \refinerpromptcard{user_prompt_eureka}{appendix/generated/prompt_skill.tex}{270}{351}%
}

\@namedef{refinerpromptcards@coderefiner}{%
  \refinerpromptcard{system_prompt_coderefiner}{appendix/generated/prompt_skill.tex}{358}{440}%
  \refinerpromptcard{user_prompt_coderefiner}{appendix/generated/prompt_skill.tex}{443}{548}%
  \refinerpromptcard{user_prompt_coderefiner_phase_1}{appendix/generated/prompt_skill.tex}{555}{592}%
  \refinerpromptcard{user_prompt_coderefiner_phase_2}{appendix/generated/prompt_skill.tex}{595}{636}%
  \refinerpromptcard{user_prompt_coderefiner_phase_3}{appendix/generated/prompt_skill.tex}{639}{760}%
  \refinerpromptcard{user_prompt_coderefiner_phase_4}{appendix/generated/prompt_skill.tex}{763}{794}%
}

\@namedef{refinerpromptcards@ablation-holistic}{%
  \refinerpromptcard{user_prompt_coderefiner_holistic}{appendix/generated/prompt_ablation_holistic.tex}{477}{511}%
}

\@namedef{refinerpromptcards@ablation-no-diagnosis}{%
  \refinerpromptcard{system_prompt_thought_obs_summarizer_chunk (plain)}{appendix/generated/prompt_ablation_no_diagnosis.tex}{46}{61}%
  \refinerpromptcard{user_prompt_thought_obs_summarizer_chunk (plain)}{appendix/generated/prompt_ablation_no_diagnosis.tex}{64}{75}%
}

\makeatother
